# Supplementary material for: GLOW: Global Illumination-Aware Inverse Rendering of Indoor Scenes Captured with Dynamic Co-Located Light & Camera
Source: arXiv:2511.22857 source file (2026-09-22)
Supplement: Supplementary file 1 [file suppl_qualitative_figure_real_generated.tex]

% Real scenes
{\makebox[5pt]{\rotatebox{90}{\footnotesize \hspace{15pt} Shoe Rack}}} &
\includegraphics[width=\width]{images/supp_fig/shoe_shelf_vignetting/rerender/5_iron.jpg} &
\includegraphics[width=\width]{images/supp_fig/shoe_shelf_vignetting/rerender/5_wildlight.jpg} &
\includegraphics[width=\width]{images/supp_fig/shoe_shelf_vignetting/rerender/5_nerad.jpg} &
\includegraphics[width=\width]{images/supp_fig/shoe_shelf_vignetting/rerender/5_gt.jpg} &
 &
{\makebox[5pt]{\rotatebox{90}{\footnotesize \hspace{15pt} Shoe Rack}}} &
\includegraphics[width=\width]{images/supp_fig/shoe_shelf_vignetting/rerender/8_iron.jpg} &
\includegraphics[width=\width]{images/supp_fig/shoe_shelf_vignetting/rerender/8_wildlight.jpg} &
\includegraphics[width=\width]{images/supp_fig/shoe_shelf_vignetting/rerender/8_nerad.jpg} &
\includegraphics[width=\width]{images/supp_fig/shoe_shelf_vignetting/rerender/8_gt.jpg} \\
{\makebox[5pt]{\rotatebox{90}{\footnotesize Albedo}}} &
\includegraphics[width=\width]{images/supp_fig/shoe_shelf_vignetting/albedo/5_iron.jpg} &
\includegraphics[width=\width]{images/supp_fig/shoe_shelf_vignetting/albedo/5_wildlight.jpg} &
\includegraphics[width=\width]{images/supp_fig/shoe_shelf_vignetting/albedo/5_nerad.jpg} &
 &
 &
{\makebox[5pt]{\rotatebox{90}{\footnotesize Albedo}}} &
\includegraphics[width=\width]{images/supp_fig/shoe_shelf_vignetting/albedo/8_iron.jpg} &
\includegraphics[width=\width]{images/supp_fig/shoe_shelf_vignetting/albedo/8_wildlight.jpg} &
\includegraphics[width=\width]{images/supp_fig/shoe_shelf_vignetting/albedo/8_nerad.jpg} &
 \\
{\makebox[5pt]{\rotatebox{90}{\footnotesize Roughness}}} &
\includegraphics[width=\width]{images/supp_fig/shoe_shelf_vignetting/roughness/5_iron.jpg} &
\includegraphics[width=\width]{images/supp_fig/shoe_shelf_vignetting/roughness/5_wildlight.jpg} &
\includegraphics[width=\width]{images/supp_fig/shoe_shelf_vignetting/roughness/5_nerad.jpg} &
 &
 &
{\makebox[5pt]{\rotatebox{90}{\footnotesize Roughness}}} &
\includegraphics[width=\width]{images/supp_fig/shoe_shelf_vignetting/roughness/8_iron.jpg} &
\includegraphics[width=\width]{images/supp_fig/shoe_shelf_vignetting/roughness/8_wildlight.jpg} &
\includegraphics[width=\width]{images/supp_fig/shoe_shelf_vignetting/roughness/8_nerad.jpg} &
 \\
{\makebox[5pt]{\rotatebox{90}{\footnotesize \hspace{24pt} Table}}} &
\includegraphics[width=\width]{images/supp_fig/irb_4th_printer_scene_vignetting_real/rerender/7_iron.jpg} &
\includegraphics[width=\width]{images/supp_fig/irb_4th_printer_scene_vignetting_real/rerender/7_wildlight.jpg} &
\includegraphics[width=\width]{images/supp_fig/irb_4th_printer_scene_vignetting_real/rerender/7_nerad.jpg} &
\includegraphics[width=\width]{images/supp_fig/irb_4th_printer_scene_vignetting_real/rerender/7_gt.jpg} &
 &
{\makebox[5pt]{\rotatebox{90}{\footnotesize \hspace{24pt} Table}}} &
\includegraphics[width=\width]{images/supp_fig/irb_4th_printer_scene_vignetting_real/rerender/34_iron.jpg} &
\includegraphics[width=\width]{images/supp_fig/irb_4th_printer_scene_vignetting_real/rerender/34_wildlight.jpg} &
\includegraphics[width=\width]{images/supp_fig/irb_4th_printer_scene_vignetting_real/rerender/34_nerad.jpg} &
\includegraphics[width=\width]{images/supp_fig/irb_4th_printer_scene_vignetting_real/rerender/34_gt.jpg} \\
{\makebox[5pt]{\rotatebox{90}{\footnotesize Albedo}}} &
\includegraphics[width=\width]{images/supp_fig/irb_4th_printer_scene_vignetting_real/albedo/7_iron.jpg} &
\includegraphics[width=\width]{images/supp_fig/irb_4th_printer_scene_vignetting_real/albedo/7_wildlight.jpg} &
\includegraphics[width=\width]{images/supp_fig/irb_4th_printer_scene_vignetting_real/albedo/7_nerad.jpg} &
 &
 &
{\makebox[5pt]{\rotatebox{90}{\footnotesize Albedo}}} &
\includegraphics[width=\width]{images/supp_fig/irb_4th_printer_scene_vignetting_real/albedo/34_iron.jpg} &
\includegraphics[width=\width]{images/supp_fig/irb_4th_printer_scene_vignetting_real/albedo/34_wildlight.jpg} &
\includegraphics[width=\width]{images/supp_fig/irb_4th_printer_scene_vignetting_real/albedo/34_nerad.jpg} &
 \\
{\makebox[5pt]{\rotatebox{90}{\footnotesize Roughness}}} &
\includegraphics[width=\width]{images/supp_fig/irb_4th_printer_scene_vignetting_real/roughness/7_iron.jpg} &
\includegraphics[width=\width]{images/supp_fig/irb_4th_printer_scene_vignetting_real/roughness/7_wildlight.jpg} &
\includegraphics[width=\width]{images/supp_fig/irb_4th_printer_scene_vignetting_real/roughness/7_nerad.jpg} &
 &
 &
{\makebox[5pt]{\rotatebox{90}{\footnotesize Roughness}}} &
\includegraphics[width=\width]{images/supp_fig/irb_4th_printer_scene_vignetting_real/roughness/34_iron.jpg} &
\includegraphics[width=\width]{images/supp_fig/irb_4th_printer_scene_vignetting_real/roughness/34_wildlight.jpg} &
\includegraphics[width=\width]{images/supp_fig/irb_4th_printer_scene_vignetting_real/roughness/34_nerad.jpg} &
 \\
{\makebox[5pt]{\rotatebox{90}{\footnotesize \hspace{-2pt} Window Sill}}} &
\includegraphics[width=\width]{images/supp_fig/home_staged_window/rerender/10_iron.jpg} &
\includegraphics[width=\width]{images/supp_fig/home_staged_window/rerender/10_wildlight.jpg} &
\includegraphics[width=\width]{images/supp_fig/home_staged_window/rerender/10_nerad.jpg} &
\includegraphics[width=\width]{images/supp_fig/home_staged_window/rerender/10_gt.jpg} &
 &
{\makebox[5pt]{\rotatebox{90}{\footnotesize \hspace{-2pt} Window Sill}}} &
\includegraphics[width=\width]{images/supp_fig/home_staged_window/rerender/22_iron.jpg} &
\includegraphics[width=\width]{images/supp_fig/home_staged_window/rerender/22_wildlight.jpg} &
\includegraphics[width=\width]{images/supp_fig/home_staged_window/rerender/22_nerad.jpg} &
\includegraphics[width=\width]{images/supp_fig/home_staged_window/rerender/22_gt.jpg} \\
{\makebox[5pt]{\rotatebox{90}{\footnotesize Albedo}}} &
\includegraphics[width=\width]{images/supp_fig/home_staged_window/albedo/10_iron.jpg} &
\includegraphics[width=\width]{images/supp_fig/home_staged_window/albedo/10_wildlight.jpg} &
\includegraphics[width=\width]{images/supp_fig/home_staged_window/albedo/10_nerad.jpg} &
 &
 &
{\makebox[5pt]{\rotatebox{90}{\footnotesize Albedo}}} &
\includegraphics[width=\width]{images/supp_fig/home_staged_window/albedo/22_iron.jpg} &
\includegraphics[width=\width]{images/supp_fig/home_staged_window/albedo/22_wildlight.jpg} &
\includegraphics[width=\width]{images/supp_fig/home_staged_window/albedo/22_nerad.jpg} &
 \\
{\makebox[5pt]{\rotatebox{90}{\footnotesize Roughness}}} &
\includegraphics[width=\width]{images/supp_fig/home_staged_window/roughness/10_iron.jpg} &
\includegraphics[width=\width]{images/supp_fig/home_staged_window/roughness/10_wildlight.jpg} &
\includegraphics[width=\width]{images/supp_fig/home_staged_window/roughness/10_nerad.jpg} &
 &
 &
{\makebox[5pt]{\rotatebox{90}{\footnotesize Roughness}}} &
\includegraphics[width=\width]{images/supp_fig/home_staged_window/roughness/22_iron.jpg} &
\includegraphics[width=\width]{images/supp_fig/home_staged_window/roughness/22_wildlight.jpg} &
\includegraphics[width=\width]{images/supp_fig/home_staged_window/roughness/22_nerad.jpg} &
 \\
