# Supplementary material for: GLOW: Global Illumination-Aware Inverse Rendering of Indoor Scenes Captured with Dynamic Co-Located Light & Camera
Source: arXiv:2511.22857 source file (2026-09-22)
Supplement: Supplementary file 2 [file suppl_qualitative_figure_synthetic_generated.tex]

% Synthetic scenes
{\makebox[5pt]{\rotatebox{90}{\textbf{\hspace{10pt} Bedroom}}}} &
\includegraphics[width=\width]{images/supp_fig/colloc-bedroom-1/rerender/12_iron.jpg} &
\includegraphics[width=\width]{images/supp_fig/colloc-bedroom-1/rerender/12_wildlight.jpg} &
\includegraphics[width=\width]{images/supp_fig/colloc-bedroom-1/rerender/12_nerad.jpg} &
\includegraphics[width=\width]{images/supp_fig/colloc-bedroom-1/rerender/12_gt.jpg} \\
{\makebox[5pt]{\rotatebox{90}{\textbf{Albedo}}}} &
\includegraphics[width=\width]{images/supp_fig/colloc-bedroom-1/albedo/12_iron.jpg} &
\includegraphics[width=\width]{images/supp_fig/colloc-bedroom-1/albedo/12_wildlight.jpg} &
\includegraphics[width=\width]{images/supp_fig/colloc-bedroom-1/albedo/12_nerad.jpg} &
\includegraphics[width=\width]{images/supp_fig/colloc-bedroom-1/albedo/12_gt.jpg} \\
{\makebox[5pt]{\rotatebox{90}{\textbf{Roughness}}}} &
\includegraphics[width=\width]{images/supp_fig/colloc-bedroom-1/roughness/12_iron.jpg} &
\includegraphics[width=\width]{images/supp_fig/colloc-bedroom-1/roughness/12_wildlight.jpg} &
\includegraphics[width=\width]{images/supp_fig/colloc-bedroom-1/roughness/12_nerad.jpg} &
\includegraphics[width=\width]{images/supp_fig/colloc-bedroom-1/roughness/12_gt.jpg} \\
{\makebox[5pt]{\rotatebox{90}{\textbf{\hspace{10pt} Bedroom}}}} &
\includegraphics[width=\width]{images/supp_fig/colloc-bedroom-1/rerender/14_iron.jpg} &
\includegraphics[width=\width]{images/supp_fig/colloc-bedroom-1/rerender/14_wildlight.jpg} &
\includegraphics[width=\width]{images/supp_fig/colloc-bedroom-1/rerender/14_nerad.jpg} &
\includegraphics[width=\width]{images/supp_fig/colloc-bedroom-1/rerender/14_gt.jpg} \\
{\makebox[5pt]{\rotatebox{90}{\textbf{Albedo}}}} &
\includegraphics[width=\width]{images/supp_fig/colloc-bedroom-1/albedo/14_iron.jpg} &
\includegraphics[width=\width]{images/supp_fig/colloc-bedroom-1/albedo/14_wildlight.jpg} &
\includegraphics[width=\width]{images/supp_fig/colloc-bedroom-1/albedo/14_nerad.jpg} &
\includegraphics[width=\width]{images/supp_fig/colloc-bedroom-1/albedo/14_gt.jpg} \\
{\makebox[5pt]{\rotatebox{90}{\textbf{Roughness}}}} &
\includegraphics[width=\width]{images/supp_fig/colloc-bedroom-1/roughness/14_iron.jpg} &
\includegraphics[width=\width]{images/supp_fig/colloc-bedroom-1/roughness/14_wildlight.jpg} &
\includegraphics[width=\width]{images/supp_fig/colloc-bedroom-1/roughness/14_nerad.jpg} &
\includegraphics[width=\width]{images/supp_fig/colloc-bedroom-1/roughness/14_gt.jpg} \\
{\makebox[5pt]{\rotatebox{90}{\textbf{\hspace{5pt} Coffee Table}}}} &
\includegraphics[width=\width]{images/supp_fig/colloc-simplified-living-room-2/rerender/9_iron.jpg} &
\includegraphics[width=\width]{images/supp_fig/colloc-simplified-living-room-2/rerender/9_wildlight.jpg} &
\includegraphics[width=\width]{images/supp_fig/colloc-simplified-living-room-2/rerender/9_nerad.jpg} &
\includegraphics[width=\width]{images/supp_fig/colloc-simplified-living-room-2/rerender/9_gt.jpg} \\
{\makebox[5pt]{\rotatebox{90}{\textbf{Albedo}}}} &
\includegraphics[width=\width]{images/supp_fig/colloc-simplified-living-room-2/albedo/9_iron.jpg} &
\includegraphics[width=\width]{images/supp_fig/colloc-simplified-living-room-2/albedo/9_wildlight.jpg} &
\includegraphics[width=\width]{images/supp_fig/colloc-simplified-living-room-2/albedo/9_nerad.jpg} &
\includegraphics[width=\width]{images/supp_fig/colloc-simplified-living-room-2/albedo/9_gt.jpg} \\
{\makebox[5pt]{\rotatebox{90}{\textbf{Roughness}}}} &
\includegraphics[width=\width]{images/supp_fig/colloc-simplified-living-room-2/roughness/9_iron.jpg} &
\includegraphics[width=\width]{images/supp_fig/colloc-simplified-living-room-2/roughness/9_wildlight.jpg} &
\includegraphics[width=\width]{images/supp_fig/colloc-simplified-living-room-2/roughness/9_nerad.jpg} &
\includegraphics[width=\width]{images/supp_fig/colloc-simplified-living-room-2/roughness/9_gt.jpg} \\
{\makebox[5pt]{\rotatebox{90}{\textbf{\hspace{5pt} Coffee Table}}}} &
\includegraphics[width=\width]{images/supp_fig/colloc-simplified-living-room-2/rerender/21_iron.jpg} &
\includegraphics[width=\width]{images/supp_fig/colloc-simplified-living-room-2/rerender/21_wildlight.jpg} &
\includegraphics[width=\width]{images/supp_fig/colloc-simplified-living-room-2/rerender/21_nerad.jpg} &
\includegraphics[width=\width]{images/supp_fig/colloc-simplified-living-room-2/rerender/21_gt.jpg} \\
{\makebox[5pt]{\rotatebox{90}{\textbf{Albedo}}}} &
\includegraphics[width=\width]{images/supp_fig/colloc-simplified-living-room-2/albedo/21_iron.jpg} &
\includegraphics[width=\width]{images/supp_fig/colloc-simplified-living-room-2/albedo/21_wildlight.jpg} &
\includegraphics[width=\width]{images/supp_fig/colloc-simplified-living-room-2/albedo/21_nerad.jpg} &
\includegraphics[width=\width]{images/supp_fig/colloc-simplified-living-room-2/albedo/21_gt.jpg} \\
{\makebox[5pt]{\rotatebox{90}{\textbf{Roughness}}}} &
\includegraphics[width=\width]{images/supp_fig/colloc-simplified-living-room-2/roughness/21_iron.jpg} &
\includegraphics[width=\width]{images/supp_fig/colloc-simplified-living-room-2/roughness/21_wildlight.jpg} &
\includegraphics[width=\width]{images/supp_fig/colloc-simplified-living-room-2/roughness/21_nerad.jpg} &
\includegraphics[width=\width]{images/supp_fig/colloc-simplified-living-room-2/roughness/21_gt.jpg} \\
{\makebox[5pt]{\rotatebox{90}{\textbf{\hspace{12pt} Shelf}}}} &
\includegraphics[width=\width]{images/supp_fig/colloc-living-room-1/rerender/5_iron.jpg} &
\includegraphics[width=\width]{images/supp_fig/colloc-living-room-1/rerender/5_wildlight.jpg} &
\includegraphics[width=\width]{images/supp_fig/colloc-living-room-1/rerender/5_nerad.jpg} &
\includegraphics[width=\width]{images/supp_fig/colloc-living-room-1/rerender/5_gt.jpg} \\
{\makebox[5pt]{\rotatebox{90}{\textbf{Albedo}}}} &
\includegraphics[width=\width]{images/supp_fig/colloc-living-room-1/albedo/5_iron.jpg} &
\includegraphics[width=\width]{images/supp_fig/colloc-living-room-1/albedo/5_wildlight.jpg} &
\includegraphics[width=\width]{images/supp_fig/colloc-living-room-1/albedo/5_nerad.jpg} &
\includegraphics[width=\width]{images/supp_fig/colloc-living-room-1/albedo/5_gt.jpg} \\
{\makebox[5pt]{\rotatebox{90}{\textbf{Roughness}}}} &
\includegraphics[width=\width]{images/supp_fig/colloc-living-room-1/roughness/5_iron.jpg} &
\includegraphics[width=\width]{images/supp_fig/colloc-living-room-1/roughness/5_wildlight.jpg} &
\includegraphics[width=\width]{images/supp_fig/colloc-living-room-1/roughness/5_nerad.jpg} &
\includegraphics[width=\width]{images/supp_fig/colloc-living-room-1/roughness/5_gt.jpg} \\
{\makebox[5pt]{\rotatebox{90}{\textbf{\hspace{12pt} Shelf}}}} &
\includegraphics[width=\width]{images/supp_fig/colloc-living-room-1/rerender/14_iron.jpg} &
\includegraphics[width=\width]{images/supp_fig/colloc-living-room-1/rerender/14_wildlight.jpg} &
\includegraphics[width=\width]{images/supp_fig/colloc-living-room-1/rerender/14_nerad.jpg} &
\includegraphics[width=\width]{images/supp_fig/colloc-living-room-1/rerender/14_gt.jpg} \\
{\makebox[5pt]{\rotatebox{90}{\textbf{Albedo}}}} &
\includegraphics[width=\width]{images/supp_fig/colloc-living-room-1/albedo/14_iron.jpg} &
\includegraphics[width=\width]{images/supp_fig/colloc-living-room-1/albedo/14_wildlight.jpg} &
\includegraphics[width=\width]{images/supp_fig/colloc-living-room-1/albedo/14_nerad.jpg} &
\includegraphics[width=\width]{images/supp_fig/colloc-living-room-1/albedo/14_gt.jpg} \\
{\makebox[5pt]{\rotatebox{90}{\textbf{Roughness}}}} &
\includegraphics[width=\width]{images/supp_fig/colloc-living-room-1/roughness/14_iron.jpg} &
\includegraphics[width=\width]{images/supp_fig/colloc-living-room-1/roughness/14_wildlight.jpg} &
\includegraphics[width=\width]{images/supp_fig/colloc-living-room-1/roughness/14_nerad.jpg} &
\includegraphics[width=\width]{images/supp_fig/colloc-living-room-1/roughness/14_gt.jpg} \\
{\makebox[5pt]{\rotatebox{90}{\textbf{\hspace{-3pt} Kitchen Counter}}}} &
\includegraphics[width=\width]{images/supp_fig/custom_kitchen_ver9_principled_path/rerender/1_iron.jpg} &
\includegraphics[width=\width]{images/supp_fig/custom_kitchen_ver9_principled_path/rerender/1_wildlight.jpg} &
\includegraphics[width=\width]{images/supp_fig/custom_kitchen_ver9_principled_path/rerender/1_nerad.jpg} &
\includegraphics[width=\width]{images/supp_fig/custom_kitchen_ver9_principled_path/rerender/1_gt.jpg} \\
{\makebox[5pt]{\rotatebox{90}{\textbf{Albedo}}}} &
\includegraphics[width=\width]{images/supp_fig/custom_kitchen_ver9_principled_path/albedo/1_iron.jpg} &
\includegraphics[width=\width]{images/supp_fig/custom_kitchen_ver9_principled_path/albedo/1_wildlight.jpg} &
\includegraphics[width=\width]{images/supp_fig/custom_kitchen_ver9_principled_path/albedo/1_nerad.jpg} &
\includegraphics[width=\width]{images/supp_fig/custom_kitchen_ver9_principled_path/albedo/1_gt.jpg} \\
{\makebox[5pt]{\rotatebox{90}{\textbf{Roughness}}}} &
\includegraphics[width=\width]{images/supp_fig/custom_kitchen_ver9_principled_path/roughness/1_iron.jpg} &
\includegraphics[width=\width]{images/supp_fig/custom_kitchen_ver9_principled_path/roughness/1_wildlight.jpg} &
\includegraphics[width=\width]{images/supp_fig/custom_kitchen_ver9_principled_path/roughness/1_nerad.jpg} &
\includegraphics[width=\width]{images/supp_fig/custom_kitchen_ver9_principled_path/roughness/1_gt.jpg} \\
{\makebox[5pt]{\rotatebox{90}{\textbf{\hspace{-3pt} Kitchen Counter}}}} &
\includegraphics[width=\width]{images/supp_fig/custom_kitchen_ver9_principled_path/rerender/8_iron.jpg} &
\includegraphics[width=\width]{images/supp_fig/custom_kitchen_ver9_principled_path/rerender/8_wildlight.jpg} &
\includegraphics[width=\width]{images/supp_fig/custom_kitchen_ver9_principled_path/rerender/8_nerad.jpg} &
\includegraphics[width=\width]{images/supp_fig/custom_kitchen_ver9_principled_path/rerender/8_gt.jpg} \\
{\makebox[5pt]{\rotatebox{90}{\textbf{Albedo}}}} &
\includegraphics[width=\width]{images/supp_fig/custom_kitchen_ver9_principled_path/albedo/8_iron.jpg} &
\includegraphics[width=\width]{images/supp_fig/custom_kitchen_ver9_principled_path/albedo/8_wildlight.jpg} &
\includegraphics[width=\width]{images/supp_fig/custom_kitchen_ver9_principled_path/albedo/8_nerad.jpg} &
\includegraphics[width=\width]{images/supp_fig/custom_kitchen_ver9_principled_path/albedo/8_gt.jpg} \\
{\makebox[5pt]{\rotatebox{90}{\textbf{Roughness}}}} &
\includegraphics[width=\width]{images/supp_fig/custom_kitchen_ver9_principled_path/roughness/8_iron.jpg} &
\includegraphics[width=\width]{images/supp_fig/custom_kitchen_ver9_principled_path/roughness/8_wildlight.jpg} &
\includegraphics[width=\width]{images/supp_fig/custom_kitchen_ver9_principled_path/roughness/8_nerad.jpg} &
\includegraphics[width=\width]{images/supp_fig/custom_kitchen_ver9_principled_path/roughness/8_gt.jpg} \\
