# Supplementary material for: GLOW: Global Illumination-Aware Inverse Rendering of Indoor Scenes Captured with Dynamic Co-Located Light & Camera
Source: arXiv:2511.22857 source file (2026-09-22)
Supplement: Supplementary file 3 [file suppl_qualitative_path_generated_real_0.tex]

% Real scenes
{\makebox[5pt]{\rotatebox{90}{\textbf{\hspace{15pt} Shoe Rack}}}} &
\includegraphics[width=\width]{images/supp_fig_path/shoe_shelf_vignetting/006_iron.jpg} &
\includegraphics[width=\width]{images/supp_fig_path/shoe_shelf_vignetting/006_wildlight.jpg} &
\includegraphics[width=\width]{images/supp_fig_path/shoe_shelf_vignetting/006_nerad.jpg} &
\includegraphics[width=\width]{images/supp_fig_path/shoe_shelf_vignetting/006_gt.jpg} \\
{\makebox[5pt]{\rotatebox{90}{\textbf{\hspace{15pt} Shoe Rack}}}} &
\includegraphics[width=\width]{images/supp_fig_path/shoe_shelf_vignetting/020_iron.jpg} &
\includegraphics[width=\width]{images/supp_fig_path/shoe_shelf_vignetting/020_wildlight.jpg} &
\includegraphics[width=\width]{images/supp_fig_path/shoe_shelf_vignetting/020_nerad.jpg} &
\includegraphics[width=\width]{images/supp_fig_path/shoe_shelf_vignetting/020_gt.jpg} \\
