# Supplementary material for: GLOW: Global Illumination-Aware Inverse Rendering of Indoor Scenes Captured with Dynamic Co-Located Light & Camera
Source: arXiv:2511.22857 source file (2026-09-22)
Supplement: Supplementary file 4 [file suppl_qualitative_path_generated_real_1.tex]

% Real scenes
{\makebox[5pt]{\rotatebox{90}{\textbf{\hspace{24pt} Table}}}} &
\includegraphics[width=\width]{images/supp_fig_path/irb_4th_printer_scene_vignetting_real/023_iron.jpg} &
\includegraphics[width=\width]{images/supp_fig_path/irb_4th_printer_scene_vignetting_real/023_wildlight.jpg} &
\includegraphics[width=\width]{images/supp_fig_path/irb_4th_printer_scene_vignetting_real/023_nerad.jpg} &
\includegraphics[width=\width]{images/supp_fig_path/irb_4th_printer_scene_vignetting_real/023_gt.jpg} \\
{\makebox[5pt]{\rotatebox{90}{\textbf{\hspace{24pt} Table}}}} &
\includegraphics[width=\width]{images/supp_fig_path/irb_4th_printer_scene_vignetting_real/028_iron.jpg} &
\includegraphics[width=\width]{images/supp_fig_path/irb_4th_printer_scene_vignetting_real/028_wildlight.jpg} &
\includegraphics[width=\width]{images/supp_fig_path/irb_4th_printer_scene_vignetting_real/028_nerad.jpg} &
\includegraphics[width=\width]{images/supp_fig_path/irb_4th_printer_scene_vignetting_real/028_gt.jpg} \\
