# Supplementary material for: GLOW: Global Illumination-Aware Inverse Rendering of Indoor Scenes Captured with Dynamic Co-Located Light & Camera
Source: arXiv:2511.22857 source file (2026-09-22)
Supplement: Supplementary file 5 [file suppl_qualitative_path_generated_real_2.tex]

% Real scenes
{\makebox[5pt]{\rotatebox{90}{\textbf{\hspace{-2pt} Window Sill}}}} &
\includegraphics[width=\width]{images/supp_fig_path/home_staged_window/021_iron.jpg} &
\includegraphics[width=\width]{images/supp_fig_path/home_staged_window/021_wildlight.jpg} &
\includegraphics[width=\width]{images/supp_fig_path/home_staged_window/021_nerad.jpg} &
\includegraphics[width=\width]{images/supp_fig_path/home_staged_window/021_gt.jpg} \\
{\makebox[5pt]{\rotatebox{90}{\textbf{\hspace{-2pt} Window Sill}}}} &
\includegraphics[width=\width]{images/supp_fig_path/home_staged_window/036_iron.jpg} &
\includegraphics[width=\width]{images/supp_fig_path/home_staged_window/036_wildlight.jpg} &
\includegraphics[width=\width]{images/supp_fig_path/home_staged_window/036_nerad.jpg} &
\includegraphics[width=\width]{images/supp_fig_path/home_staged_window/036_gt.jpg} \\
