# Supplementary material for: GLOW: Global Illumination-Aware Inverse Rendering of Indoor Scenes Captured with Dynamic Co-Located Light & Camera
Source: arXiv:2511.22857 source file (2026-09-22)
Supplement: Supplementary file 6 [file suppl_qualitative_path_generated_synthetic_0.tex]

% Synthetic scenes 0
{\makebox[5pt]{\rotatebox{90}{\textbf{\hspace{10pt} Bedroom}}}} &
\includegraphics[width=\width]{images/supp_fig_path/colloc-bedroom-1/000_iron.jpg} &
\includegraphics[width=\width]{images/supp_fig_path/colloc-bedroom-1/000_wildlight.jpg} &
\includegraphics[width=\width]{images/supp_fig_path/colloc-bedroom-1/000_nerad.jpg} &
\includegraphics[width=\width]{images/supp_fig_path/colloc-bedroom-1/000_gt.jpg} \\
{\makebox[5pt]{\rotatebox{90}{\textbf{\hspace{10pt} Bedroom}}}} &
\includegraphics[width=\width]{images/supp_fig_path/colloc-bedroom-1/012_iron.jpg} &
\includegraphics[width=\width]{images/supp_fig_path/colloc-bedroom-1/012_wildlight.jpg} &
\includegraphics[width=\width]{images/supp_fig_path/colloc-bedroom-1/012_nerad.jpg} &
\includegraphics[width=\width]{images/supp_fig_path/colloc-bedroom-1/012_gt.jpg} \\
