# Supplementary material for: GLOW: Global Illumination-Aware Inverse Rendering of Indoor Scenes Captured with Dynamic Co-Located Light & Camera
Source: arXiv:2511.22857 source file (2026-09-22)
Supplement: Supplementary file 7 [file suppl_qualitative_path_generated_synthetic_1.tex]

% Synthetic scenes 1
{\makebox[5pt]{\rotatebox{90}{\textbf{\hspace{5pt} Coffee Table}}}} &
\includegraphics[width=\width]{images/supp_fig_path/colloc-simplified-living-room-2/001_iron.jpg} &
\includegraphics[width=\width]{images/supp_fig_path/colloc-simplified-living-room-2/001_wildlight.jpg} &
\includegraphics[width=\width]{images/supp_fig_path/colloc-simplified-living-room-2/001_nerad.jpg} &
\includegraphics[width=\width]{images/supp_fig_path/colloc-simplified-living-room-2/001_gt.jpg} \\
{\makebox[5pt]{\rotatebox{90}{\textbf{\hspace{5pt} Coffee Table}}}} &
\includegraphics[width=\width]{images/supp_fig_path/colloc-simplified-living-room-2/009_iron.jpg} &
\includegraphics[width=\width]{images/supp_fig_path/colloc-simplified-living-room-2/009_wildlight.jpg} &
\includegraphics[width=\width]{images/supp_fig_path/colloc-simplified-living-room-2/009_nerad.jpg} &
\includegraphics[width=\width]{images/supp_fig_path/colloc-simplified-living-room-2/009_gt.jpg} \\
