# Supplementary material for: GLOW: Global Illumination-Aware Inverse Rendering of Indoor Scenes Captured with Dynamic Co-Located Light & Camera
Source: arXiv:2511.22857 source file (2026-09-22)
Supplement: Supplementary file 8 [file suppl_qualitative_path_generated_synthetic_2.tex]

% Synthetic scenes 2
{\makebox[5pt]{\rotatebox{90}{\textbf{\hspace{12pt} Shelf}}}} &
\includegraphics[width=\width]{images/supp_fig_path/colloc-living-room-1/007_iron.jpg} &
\includegraphics[width=\width]{images/supp_fig_path/colloc-living-room-1/007_wildlight.jpg} &
\includegraphics[width=\width]{images/supp_fig_path/colloc-living-room-1/007_nerad.jpg} &
\includegraphics[width=\width]{images/supp_fig_path/colloc-living-room-1/007_gt.jpg} \\
{\makebox[5pt]{\rotatebox{90}{\textbf{\hspace{12pt} Shelf}}}} &
\includegraphics[width=\width]{images/supp_fig_path/colloc-living-room-1/008_iron.jpg} &
\includegraphics[width=\width]{images/supp_fig_path/colloc-living-room-1/008_wildlight.jpg} &
\includegraphics[width=\width]{images/supp_fig_path/colloc-living-room-1/008_nerad.jpg} &
\includegraphics[width=\width]{images/supp_fig_path/colloc-living-room-1/008_gt.jpg} \\
