# Supplementary material for: GLOW: Global Illumination-Aware Inverse Rendering of Indoor Scenes Captured with Dynamic Co-Located Light & Camera
Source: arXiv:2511.22857 source file (2026-09-22)
Supplement: Supplementary file 9 [file suppl_qualitative_path_generated_synthetic_3.tex]

% Synthetic scenes 3
{\makebox[5pt]{\rotatebox{90}{\textbf{\hspace{-3pt} Kitchen Counter}}}} &
\includegraphics[width=\width]{images/supp_fig_path/custom_kitchen_ver9_principled_path/000_iron.jpg} &
\includegraphics[width=\width]{images/supp_fig_path/custom_kitchen_ver9_principled_path/000_wildlight.jpg} &
\includegraphics[width=\width]{images/supp_fig_path/custom_kitchen_ver9_principled_path/000_nerad.jpg} &
\includegraphics[width=\width]{images/supp_fig_path/custom_kitchen_ver9_principled_path/000_gt.jpg} \\
{\makebox[5pt]{\rotatebox{90}{\textbf{\hspace{-3pt} Kitchen Counter}}}} &
\includegraphics[width=\width]{images/supp_fig_path/custom_kitchen_ver9_principled_path/008_iron.jpg} &
\includegraphics[width=\width]{images/supp_fig_path/custom_kitchen_ver9_principled_path/008_wildlight.jpg} &
\includegraphics[width=\width]{images/supp_fig_path/custom_kitchen_ver9_principled_path/008_nerad.jpg} &
\includegraphics[width=\width]{images/supp_fig_path/custom_kitchen_ver9_principled_path/008_gt.jpg} \\
